# Supplementary material for: Chain-of-Thought Prompting Elicits Reasoning in Large Language Models
Source: arXiv:2201.11903 source file (2023-01-10)
Supplement: Supplementary file 1 [file appendix-reverse-object-prompt.tex]

\begingroup
\begin{table}[H]
    \centering
    \small
    \caption{    
    Few-shot exemplars for full chain of thought prompt for the reverse list of objects task.
    We found that prompt engineering improved performance on this task specifically (we did not do prompt engineering on any other tasks).
    }
    \begin{tabular}{p{\linewidth}}
        \toprule
        \underline{\textbf{\textsc{Prompt for Reverse List}}} \\
        \vspace{-2mm}
        \textbf{Q:} Reverse the sequence "cigar, umbrella, key, gum, alarm". \\
        \vspace{-1mm}
        \textbf{A:} \hl{First is cigar. Second is umbrella. Third is key. Fourth is gum. Fifth is alarm. Now to reverse, change the order to: Fifth is alarm. Fourth is gum. Third is key. Second is umbrella. First is cigar.} So the answer is "alarm, gum, key, umbrella, cigar". \\
        \vspace{0mm}
        \textbf{Q:} Reverse the sequence "player, passport, umbrella, bottle, watch". \\
        \vspace{-1mm}
        \textbf{A:} \hl{First is player. Second is passport. Third is umbrella. Fourth is bottle. Fifth is watch. Now to reverse, change the order to: Fifth is watch. Fourth is bottle. Third is umbrella. Second is passport. First is player.} So the answer is "watch, bottle, umbrella, passport, player". \\
        \vspace{0mm}
        \textbf{Q:} Reverse the sequence "coin, postcard, case, pen, wallet". \\
        \vspace{-1mm}
        \textbf{A:} \hl{First is coin. Second is postcard. Third is case. Fourth is pen. Fifth is wallet. Now to reverse, change the order to: Fifth is wallet. Fourth is pen. Third is case. Second is postcard. First is coin.} So the answer is "wallet, pen, case, postcard, coin". \\
        \vspace{0mm}
        \textbf{Q:} Reverse the sequence "laptop, lipstick, pen, bin, clock". \\
        \vspace{-1mm}
        \textbf{A:} \hl{First is laptop. Second is lipstick. Third is pen. Fourth is bin. Fifth is clock. Now to reverse, change the order to: Fifth is clock. Fourth is bin. Third is pen. Second is lipstick. First is laptop.} So the answer is "clock, bin, pen, lipstick, laptop". \\
        \vspace{0mm}
        \textbf{Q:} Reverse the sequence "key, pen, screen, file, cigar". \\
        \vspace{-1mm}
        \textbf{A:} \hl{First is key. Second is pen. Third is screen. Fourth is file. Fifth is cigar. Now to reverse, change the order to: Fifth is cigar. Fourth is file. Third is screen. Second is pen. First is key.} So the answer is "cigar, file, screen, pen, key". \\
        \vspace{0mm}
        \textbf{Q:} Reverse the sequence "card, stamp, book, water, glasses". \\
        \vspace{-1mm}
        \textbf{A:} \hl{First is card. Second is stamp. Third is book. Fourth is water. Fifth is glasses. Now to reverse, change the order to: Fifth is glasses. Fourth is water. Third is book. Second is stamp. First is card.} The answer is 29. \\
        \vspace{0mm}
        \textbf{Q:} Reverse the sequence "clock, coin, bottle, head, postcard". \\
        \vspace{-1mm}
        \textbf{A:} \hl{First is clock. Second is coin. Third is bottle. Fourth is head. Fifth is postcard. Now to reverse, change the order to: Fifth is postcard. Fourth is head. Third is bottle. Second is coin. First is clock.} So the answer is "postcard, head, bottle, coin, clock". \\
        \vspace{0mm}
        \textbf{Q:} Reverse the sequence "battery, glasses, lighter, water, scissors". \\
        \vspace{-1mm}
        \textbf{A:} \hl{First is battery. Second is glasses. Third is lighter. Fourth is water. Fifth is scissors. Now to reverse, change the order to: Fifth is scissors. Fourth is water. Third is lighter. Second is glasses. First is battery.} So the answer is "scissors, water, lighter, glasses, battery". \\
        \bottomrule
    \end{tabular}
    \label{tab:appendix-reverse-list-prompt}
\end{table}
\endgroup
